# Supplementary material for: Microwave to optical photon conversion via fully concentrated rare-earth ion crystals
Source: arXiv:1812.03246 ancillary file (2018-12-08)
Supplement: Supplementary file 1 [file Supplementary1.pdf]

# Physical constants

Defining physical constants for use later

In[1]:=
```
constants = {μB → 9.274 * 10^-24, h → 6.626 * 10^-34, ℏ → (6.626 * 10^-34)/(2 π), μ0 → 4 π * 10^-7,
   ϵ0 → 8.854 * 10^-12, e → 1.602 * 10^-19, m → 9.109 * 10^-31, c → 3 * 10^8};
```

# Magnetic transition dipole moment ($\mu_{g1}$)

In this section we use the known electronic g-tensor of erbium chloride hexahydrate to calculate the range of values $\mu_{g1}$ can take. The transition dipole moment is given by $|\mu_{1g}| = \frac{1}{2}\mu_B \left| \langle \psi_1 | g.\tilde{S} | \psi_g \rangle \right|$, where $g$ is the g-tensor, $\tilde{S}$ is the vector of spin operators, and $|\psi_g\rangle$, $|\psi_1\rangle$ are the eigenstates of the lower and upper Zeeman levels.

Because $g$ is anisotropic, both the Zeeman splitting and the dipole moment depends on both the magnetic field strength and direction. To investigate the range of value $\mu_{g1}$ can take, we do the following:

1) Define a set of magnetic field directions that samples many different possible directions. We take a "Longdell Spiral"

2) Define a spin hamiltonian for the two level system

3) Use the spin hamiltonian to calculate the field strength needed to produce a 5 GHz Zeeman splitting for each direction in the "Londell Spiral"

4) Use the spin hamiltonian and the magnetic fields determined in step 3 to calculate the eigenstates for each direction in the "Longdell Spiral"

5) Calculate $\mu_{g1}$ for each direction of the "Longdell Spiral"

The g-tensor used here is from the work of Couture and Rajnak, Chem. Phys. 95 315-332 (1984).

Step 1:

Let the magnetic field follow a Longdell spiral, which will sample many different directions of magnetic fields. We will consider 5000 points along the spiral

In[2]:=
```
Bx = B0 Sqrt[1.0 - t^2] Cos[6 π t];
By = B0 Sqrt[1.0 - t^2] Sin[6 π t];
Bz = B0 t;
numpoints = 5000;
ts = Table[t, {t, -1., 1, 2 / (numpoints - 1)}];
```

Step 2:

We now define the Spin Hamitonian. Because we are only interested in the range of values $\mu_{g1}$can take, we can remain in the g-tensor principal axes frame. The spin hamiltonian is given by *B.M.I*, where *B* is

the applied magnetic field vector, *M* is the Zeeman tensor, and *I* is a vector of spin operators.

In[7]:=
```
(*Define Zeeman tensor*)
gx = 13.1;
gy = 0.0;
gz = 0.55;
M = DiagonalMatrix[{gx, gy, gz}];
(*Define spin matrices*)
Ix = {{0, 1.0}, {1.0, 0}};
Iy = {{0.0, -I}, {I, 0.0}};
Iz = {{1.0, 0}, {0, -1.0}};
(*Define Spin Hamiltonian, BMI *)
{MIx, MIy, MIz} = M.{Ix, Iy, Iz};
BMI = Bx MIx + By MIy + Bz MIz;
```

Step 3:
Calculate the  Zeeman splitting from the eigenvalues of the  Spin Hamiltonian for each direction in the spiral. It is a function B0 and t.
We then calculate the value of B0 needed to produce a 5 GHz spiltting for each value of t.

In[16]:=
```
eigval = Eigenvalues[BMI];
splitting = μB/h (eigval[[2]] - eigval[[1]]) /. constants;
freqtarget = 5.0 * 10^9;
B0s = Re[Flatten[Table[{Solve[splitting == freqtarget, B0][[1, 1, 2]]}, {t, ts}]]];
```

Step 4:
Lets create a list “BMIs” which is the list of Spin Hamiltonian matrices calculated for each of the magnetic fields. We then take the eigenvectors of each matrix to get the two states for each field.

In[20]:=
```
BMIs = Table[BMI /. B0 → B0s[[ii]] /. t → ts[[ii]], {ii, 1, numpoints}];
eigvecs = Table[Eigenvectors[BMIs[[ii]]], {ii, 1, numpoints}];
```

Step 5:
The dipole moment is given by $|\mu_{1\,g}| = \frac{1}{2}\mu_B \left| \langle \psi_1 | \, g.\tilde{S} \, | \psi_g \rangle \right|$. Let’s call the x component of $g.\tilde{S}$, $gS_X$ and so on. Also, $g$ is the same as *M* and $\tilde{S} = \frac{1}{2}(I_x, I_y, I_z)$. We can now calculate the dipole moment for each direction in the Longdell Sprial. We plot the result along the spin of a free electron, as a reality check.

In[22]:=
```
{gSx, gSy, gSz} = 1/2 M.{Ix, Iy, Iz};
μ1g =
  Table[1/2 μB Abs[Conjugate[eigvecs[[ii, 1]]].Sqrt[gSx^2 + gSy^2 + gSz^2].eigvecs[[ii, 2]]],
    {ii, 1, numpoints}] /. constants;
μelectron = Table[9.28 * 10^-24, {ii, 1, numpoints}];
ListLogPlot[{μ1g, μelectron}, Joined → True, PlotRange → All,
 PlotLegends → {"|μ|", "μelectron"}, AxesLabel → {"t", "μ (J/T)"}, ImageSize → Large]
```

Out[25]=
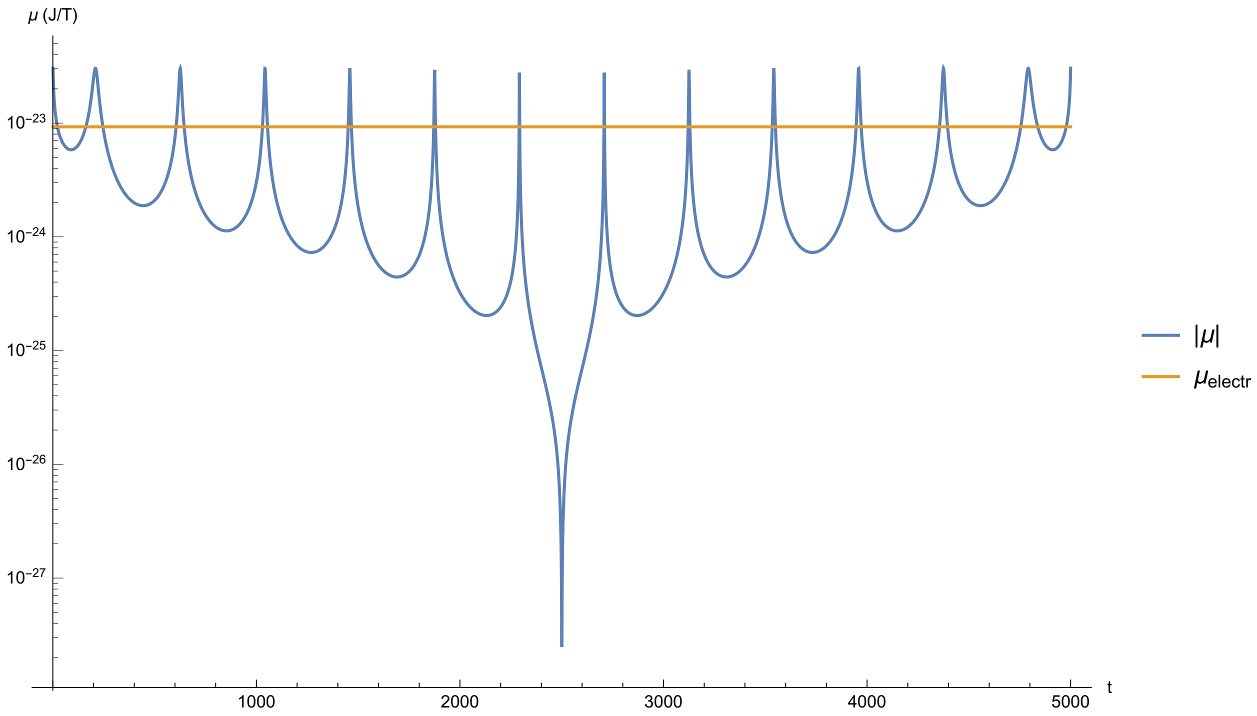


The maximum value the transition dipole takes:

In[26]:=
```
Max[μ1g]
```

Out[26]=
```
3.03724 × 10^-23
```

For our device we use $\mu_{1g} = 9.78 * 10^{-26}\ J/T$. The field required for this is:

In[27]:=
```
B0s[[First@Nearest[μ1g → Range[Length[μ1g]], 9.78 * 10^-26]]]
```

Out[27]=
```
0.0219928
```

20 mT is an experimentally feasible field.

# Electric transition dipole moment ($d_{g2}$)

In an unpulbished experiment by author R. Ahlefeldt, an oscillator strength of $1.1 * 10^{-7}$ was been measured for Erbium doped in Europium chloride hexahydrate. As this host crystal is isomorphic it our

sample, the oscillator strengths should be very similar.
We used the relation between transition dipole moment and oscillator strength given by R C Hilborn, American Jour. Phys. 50 982 (1982).

In[65]:=
```
g1 = 1; (*degeneracy of lower level*)
g2 = 1; (*degeneracy of upper level*)
f = 1.1 * 10^-7; (*oscillator strength*)
ω = 2 π * 195.5 * 10^12; (*optical angular frequency*)
```

$$dg2 = \sqrt{\frac{3}{2}\frac{g1}{g2}\frac{\hbar e^2}{\omega m} f} \text{ /. constants}$$

Out[67]= $1.99775 \times 10^{-32}$

# Rabi frequency ($\Omega_0$)

The maximum Rabi frequency is determined by the highest electric field strength in the cavity. This depends on the input power, beam cross-sectional area, refractive index, the transition dipole moment and the finesse of the cavity.
Here we use basic relations between cavity reflectance, finesse and quality to calculate the resonant enhancement of the electric field strength inside a cavity.
Relationships used are collated in N Ismail, C C Kores, D Geskus, and M Pollnau, Opt. Express 24, 16366-16389 (2016).

```
Clear[R, F, FSR, FWHM, τ, f0, Qo]
enhancement = 1/(1 - R); (*R is reflectance*)
R = Exp[-π/Finesse];
Finesse = FSR/FWHM;
(*FSR = free spectral range, FWHM = full width at half maximum *)
FWHM = 1/(π τ) (*τ is decay time of the electric field*);
fo = 195.5 * 10^12; (*fo is optical frequency*)
τ = Qo/(π fo); (*Qo is optical quality*)
L = 3.0 * 10^-2; (*L is length of cavity, 3cm = 5GHz FSR*)
FSR = c/(2 L) /. constants;
LogLogPlot[enhancement, {Qo, 1000, 6 * 10^7}, PlotRange → All,
 AxesLabel → {"Qₒ", "Field enhancement factor"}, ImageSize → Large]
```

Out[77]=

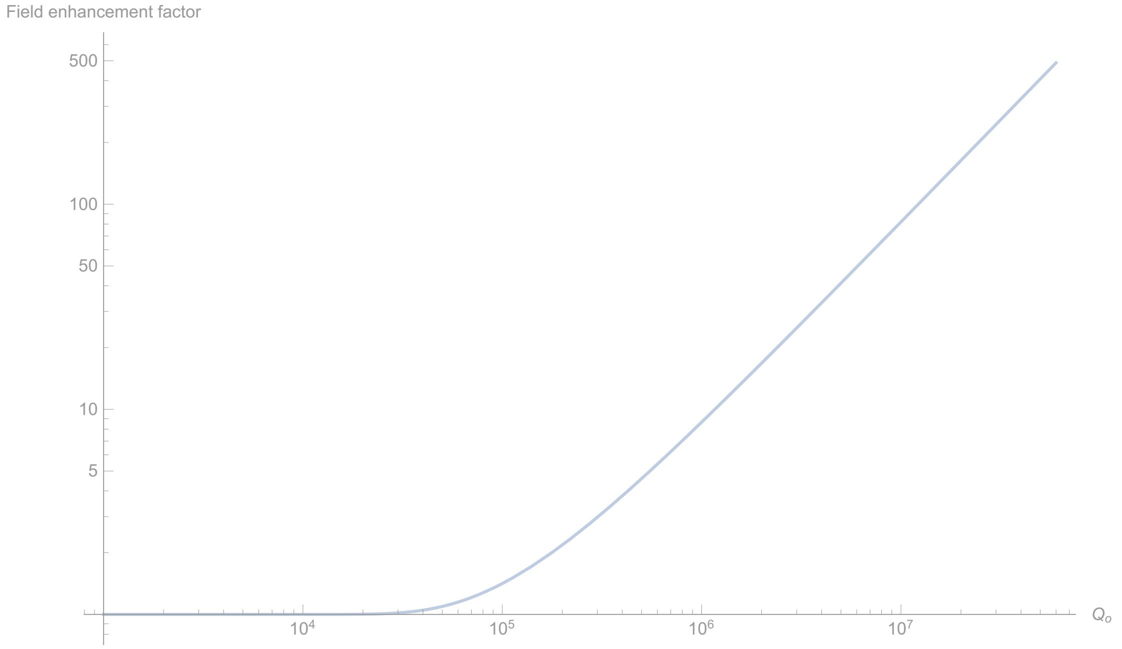


The field enhancement factor for a Fabry Perot cavity with a quality of $9.7*10^7$ is:

In[43]:=
```
enhancement /. Qo → 9.7 * 10^7
```

Out[43]= 790.169

We can now calculate the maximum Rabi frequency, which is given by $\Omega = \frac{d_{12} E}{\hbar}$ where $E$ is the maximum electric field in the sample. Assuming a maximum laser power of 1 um and a beam width of 27 um (obtained from the cavity modeling).

In[78]:=
$$E0 = \sqrt{\frac{2 P}{c\, \epsilon0\, n\, A}};$$ (*P is laser power, n is refractive index and A is beam area *)

$$\Omega = \frac{d12\ E0 * enhancement}{\hbar}\ /.\ constants\ /.$$
$$\{P \to 10^{-6},\ A \to \pi * (27 * 10^{-6})^2,\ n \to 1.58,\ Qo \to 9.7 * 10^7,\ d12 \to 2 * 10^{-32}\}$$

Out[78]= $6.8359 \times 10^7$

So a 68 MHz Rabi frequency is possible

# Cavity coupling ($G_\mu$, $G_{o,\Omega}$)

Here we calculate the maximum coupling strength of the Kittel mode to the microwave ($G_\mu$) and optical ($G_{o,\Omega}$) cavities, given by Equations 11 & 12 in the text. As described in the text, values lower then the maximum are used to ensure an adiabatic regime.

We take the most extreme but physically realistic values calculated above, and use the cavity mode volumes and filling factors calculated from the cavity models.

In[46]:= Clear[dg2]

$$extremeparameters = \{Vc \to \frac{4\pi (1 * 10^{-3})^3}{3},\ \omega\mu \to 2\pi * 5 * 10^9,$$
$$\omega o \to 2\pi * 195 * 10^{12},\ \rho \to 4 * 10^{27},\ \mu g1 \to 3 * 10^{-23},\ dg2 \to 2 * 10^{-32},$$
$$V\mu \to 2.9 * 10^{-7},\ Vo \to 2.9 * 10^{-11},\ F \to 4.7 * 10^{-4},\ \Omega 0 \to 68 * 10^6,\ \delta o \to 6.2 * 10^9\};$$

$$g\mu = \sqrt{\frac{\omega\mu\ \mu 0}{2\hbar\ V\mu}}\ \mu g1;$$

$$go = \sqrt{\frac{\omega o}{2\hbar\, \epsilon 0\, Vo}}\ dg2;$$

$$G\mu = \sqrt{\rho\, Vc}\ \sqrt{\frac{\omega\mu\ \mu 0}{2\hbar\ V\mu}}\ \mu g1;$$

$$Go = \sqrt{\rho\, Vc}\ \sqrt{\frac{\omega o}{2\hbar\, \epsilon 0\, Vo}}\ \frac{dg2\ \Omega 0}{\delta o}\ F;$$

```
Gμ /. extremeparameters /. constants
Go /. extremeparameters /. constants
```

Out[52]= $3.11979 \times 10^9$

Out[53]= $6.34756 \times 10^7$

Therefore the maximum value of $G_\mu$ is 3.1 GHz, and for $G_{o,\Omega}$ is 63 MHz.

As described in section IV the text, we propose using lesser values of $G_\mu$ = 10 MHz and $G_{o,\Omega}$ = 10 MHz.

This is achieveable with the following values:

```
In[89]:= Vc = 4 π (1 * 10^-3)^3 / 3; (*2 mm radius crystal*)
ωμ = 2 π * 5 * 10^9; (*5 GHz microwave transition*)
ωo = 2 π * 195 * 10^12 ; (*1550 nm optical transition*)
ρ = 4 * 10^27 ; (*ion concentration in erbium chloride hexahydrate*)
μg1 = 9.7 * 10^-26; (*magnetic transition dipole moment that
 exists for a 22 mT field applied in a particular direction *)
dg2 = 2 * 10^-32; (*optical transition dipole moment*)
Vμ = 2.9 * 10^-7; (*microwave cavity mode volume,
obtained from modelling proposed cavity design*)
Vo = 2.9 * 10^-11;(*optical caivty mode volume,
obtained from modelling proposed cavity design*)
F = 4.7 * 10^-4;(*cavity filling factor,
obtained from modelling proposed cavity design*)
Ω0 = 21.5 * 10^6 ;(*proposed Rabi frequency,
which only requires 0.1 uW laser power*)
δo = 12.4 * 10^9; (*optical detuning to use*)
Gμ /. constants
Go /. constants
```

Out[94]= $1.00873 \times 10^7$

Out[95]= $1.00348 \times 10^7$

# Cavity Qualities ($Q_\mu$, $Q_o$)

The impedance matching condition requires that the cavity decay rate, $\kappa$, is 2 MHz. We now can calculate the necessary cavity quality factors for this.

```
In[96]:= κ = 2.0 * 10^6;
Qμ = ωμ / (κ 2 π) /. realsiticparameters
Qo = ωo / (κ 2 π) /. realsiticparameters
```

Out[97]= 2500.

Out[98]= $9.75 \times 10^7$
